# Supplementary material for: Time-frequency analysis of event-related brain recordings: Connecting power of evoked potential and inter-trial coherence
Source: arXiv:2211.08811 ancillary file (2022-11-16)
Supplement: Supplementary file 1 [file Supplement1.pdf]

# Supplementary material #1 for manuscript “Time-frequency analysis of event-related brain recordings: Connecting power of evoked potential and inter-trial coherence”

Jonas Benhamou, Michel Le Van Quyen, and Guillaume Marrelec

## Contents

|          |                                                                      |           |
|----------|----------------------------------------------------------------------|-----------|
| <b>1</b> | <b>Expression of avgAMP, ITC, and POWavg</b>                         | <b>2</b>  |
| 1.1      | avgAMP . . . . .                                                     | 2         |
| 1.2      | ITC . . . . .                                                        | 2         |
| 1.3      | POWavg . . . . .                                                     | 2         |
| 1.4      | Summary of properties . . . . .                                      | 3         |
| <b>2</b> | <b>Investigation of oscillatory model</b>                            | <b>3</b>  |
| 2.1      | Preliminary results . . . . .                                        | 3         |
| 2.2      | S-transform of oscillatory signal . . . . .                          | 4         |
| 2.3      | Approximation . . . . .                                              | 5         |
| 2.3.1    | General approach . . . . .                                           | 5         |
| 2.3.2    | Bounds for $\epsilon_m(t, f)$ . . . . .                              | 6         |
| 2.3.3    | Bounds for $\epsilon_a(t, f)$ . . . . .                              | 6         |
| 2.3.4    | Modulus of $T_x(t, f)$ . . . . .                                     | 7         |
| 2.3.5    | Argument of $T_x(t, f)$ . . . . .                                    | 7         |
| 2.3.6    | Summary of bounds . . . . .                                          | 7         |
| 2.4      | Model with varying amplitude and phase . . . . .                     | 7         |
| 2.5      | Model with varying amplitude, frequency, and phase . . . . .         | 8         |
| 2.5.1    | Preliminary results . . . . .                                        | 8         |
| 2.5.2    | Expectation of $ T_x^\dagger(t, f) $ . . . . .                       | 10        |
| 2.5.3    | Expectation of $e^{i \arg[T_x^\dagger(t, f)]}$ . . . . .             | 10        |
| 2.5.4    | Expectation of $T_x^\dagger(t, f)$ . . . . .                         | 10        |
| 2.6      | Summary of results . . . . .                                         | 11        |
| <b>3</b> | <b>Proof of general relationship between avgAMP, ITC, and POWavg</b> | <b>11</b> |

# 1 Expression of avgAMP, ITC, and POWavg

## 1.1 avgAMP

The square of avgAMP can be expanded as

$$\begin{aligned} \text{avgAMP}_{x_{1:N}}(t, f)^2 &= \left[ \frac{1}{N} \sum_{n=1}^N |T_{x_n}(t, f)| \right]^2 \\ &= \frac{1}{N^2} \left[ \sum_{n=1}^N |T_{x_n}(t, f)|^2 + \sum_{m \neq n} |T_{x_m}(t, f)| |T_{x_n}(t, f)| \right]. \end{aligned} \quad (\text{S-1})$$

Its expectation yields

$$\begin{aligned} \mathbb{E} [\text{avgAMP}_{x_{1:N}}(t, f)^2] &= \frac{1}{N} \mathbb{E} [|T_x(t, f)|^2] + \left(1 - \frac{1}{N}\right) \mathbb{E} [|T_x(t, f)|]^2 \\ &= \mathbb{E} [|T_x(t, f)|]^2 + \frac{1}{N} \text{Var} [|T_x(t, f)|]. \end{aligned} \quad (\text{S-2})$$

## 1.2 ITC

The square of ITC can be expanded as

$$\text{ITC}_{x_{1:N}}(t, f)^2 = \frac{1}{N} + \frac{1}{N^2} \sum_{m \neq n} e^{i[\theta_{x_m}(t, f) - \theta_{x_n}(t, f)]}. \quad (\text{S-3})$$

Its expectation is given by

$$\begin{aligned} \mathbb{E} [\text{ITC}_{x_{1:N}}(t, f)^2] &= \frac{1}{N} + \left(1 - \frac{1}{N}\right) \left| \mathbb{E} [e^{i\theta_x(t, f)}] \right|^2 \\ &= \left| \mathbb{E} [e^{i\theta_x(t, f)}] \right|^2 + \frac{1}{N} \text{Var} [e^{i\theta_x(t, f)}], \end{aligned} \quad (\text{S-4})$$

where we used the fact that, according to Equation (7) of the manuscript, we have

$$\text{Var} [e^{i\theta_x(t, f)}] = 1 - \left| \mathbb{E} [e^{i\theta_x(t, f)}] \right|^2. \quad (\text{S-5})$$

## 1.3 POWavg

We have

$$\begin{aligned} \text{POWavg}_{x_{1:N}}(t, f) &= \left[ \frac{1}{N} \sum_{n=1}^N T_{x_n}(t, f) \right] \left[ \frac{1}{N} \sum_{n=1}^N T_{x_n}(t, f) \right]^* \\ &= \frac{1}{N^2} \left[ \sum_{n=1}^N |T_{x_n}(t, f)|^2 + \sum_{m \neq n} T_{x_m}(t, f) T_{x_n}(t, f)^* \right]. \end{aligned}$$

Taking the expectation yields

$$\mathbb{E} [\text{POWavg}_{x_{1:N}}(t, f)] = \frac{1}{N^2} \left\{ \sum_{n=1}^N \mathbb{E} [|T_{x_n}(t, f)|^2] + \sum_{n \neq m} \mathbb{E} [T_{x_n}(t, f) T_{x_m}(t, f)^*] \right\}.$$

Since the  $T_{x_n}(t, f)$ 's are i.i.d. realizations of  $T_x(t, f)$ , we obtain

$$\begin{aligned} \mathbb{E} [T_{x_n}(t, f) T_{x_m}(t, f)^*] &= \mathbb{E} [T_{x_n}(t, f)] \mathbb{E} [T_{x_m}(t, f)]^* \\ &= |\mathbb{E} [T_x(t, f)]|^2 \end{aligned}$$

and

$$\begin{aligned} \mathbb{E} [\text{POWavg}_{g_{x_1:N}}(t, f)] &= \frac{1}{N} \mathbb{E} [|T_x(t, f)|^2] + \left(1 - \frac{1}{N}\right) |\mathbb{E} [T_x(t, f)]|^2 \\ &= |\mathbb{E} [T_x(t, f)]|^2 + \frac{1}{N} \text{Var} [T_x(t, f)]. \end{aligned} \quad (\text{S-6})$$

## 1.4 Summary of properties

Results regarding the properties of the expectation of avgAMP<sup>2</sup>, ITC<sup>2</sup> and POWavg are summarized here.

| Measure             | Expectation              |                                        |                                                                    |
|---------------------|--------------------------|----------------------------------------|--------------------------------------------------------------------|
|                     | depends on               | limit as $N \rightarrow \infty$        | asymptotic expectation                                             |
| avgAMP <sup>2</sup> | amplitude, $ T_x(t, f) $ | $\mathbb{E} [ T_x(t, f) ^2]$           | $\mathbb{E} [ T_x(t, f) ^2] + O\left(\frac{1}{N}\right)$           |
| ITC <sup>2</sup>    | phase, $\theta_x(t, f)$  | $ \mathbb{E} [e^{i\theta_x(t, f)}] ^2$ | $ \mathbb{E} [e^{i\theta_x(t, f)}] ^2 + O\left(\frac{1}{N}\right)$ |
| POWavg              | both, $T_x(t, f)$        | $ \mathbb{E} [T_x(t, f)] ^2$           | $ \mathbb{E} [T_x(t, f)] ^2 + O\left(\frac{1}{N}\right)$           |

## 2 Investigation of oscillatory model

### 2.1 Preliminary results

We need the values of the three following integrals. The first integral is

$$I_1(t, \alpha, f) = \frac{1}{\sqrt{2\pi\alpha^2}} \int e^{-\frac{(u-t)^2}{2\alpha^2}} e^{-2i\pi fu} du. \quad (\text{S-7})$$

It can be obtained as the characteristic function of a normal distribution (Polyanin and Manzhirov, 2007, Equation (20.2.4.6)) computed at  $-2\pi f$ ,

$$I_1(t, \alpha, f) = e^{-\frac{1}{2}(2\pi\alpha f)^2} e^{-2i\pi ft}. \quad (\text{S-8})$$

The second integral is

$$I_2(\Omega, t, \alpha, f) = \frac{1}{\sqrt{2\pi\alpha^2}} \int \Omega \cos(2\pi\nu u + \phi) e^{-\frac{(u-t)^2}{2\alpha^2}} e^{-2i\pi fu} du. \quad (\text{S-9})$$

It can be computed by first using Euler formula for the cosine function (Polyanin and Manzhirov, 2007, §2.2.3-14)

$$\begin{aligned} I_2(\Omega, t, \alpha, f) &= \frac{\Omega}{\sqrt{2\pi\alpha^2}} \int \frac{e^{i(2\pi\nu u + \phi)} + e^{-i(2\pi\nu u + \phi)}}{2} e^{-\frac{(u-t)^2}{2\alpha^2}} e^{-2i\pi fu} du \\ &= \frac{\Omega}{2} e^{i\phi} \frac{1}{\sqrt{2\pi\alpha^2}} \int e^{-\frac{(u-t)^2}{2\alpha^2}} e^{-2i\pi(f-\nu)u} du + \frac{\Omega}{2} e^{-i\phi} \frac{1}{\sqrt{2\pi\alpha^2}} \int e^{-\frac{(u-t)^2}{2\alpha^2}} e^{-2i\pi(f+\nu)u} du, \end{aligned} \quad (\text{S-10})$$

and then integrating each exponential using (S-8):

$$\begin{aligned} I_2(\Omega, t, \alpha, f) &= \frac{\Omega}{2} e^{i\phi} I_1(t, \alpha, f - \nu) + \frac{\Omega}{2} e^{-i\phi} I_1(t, \alpha, f + \nu) \\ &= \frac{\Omega}{2} e^{-\frac{1}{2}(2\pi\alpha)^2(f-\nu)^2} e^{i[\phi - 2\pi(f-\nu)t]} + \frac{\Omega}{2} e^{-\frac{1}{2}(2\pi\alpha)^2(f+\nu)^2} e^{i[-\phi - 2\pi(f+\nu)t]}. \end{aligned} \quad (\text{S-11})$$

The third and last integral is

$$I_3(\Omega, t, \alpha, t_0, \tau, f) = \frac{1}{\sqrt{2\pi\alpha^2}} \int \Omega \cos(2\pi\nu u + \phi) e^{-\frac{(u-t_0)^2}{2\tau^2}} e^{-\frac{(u-t)^2}{2\alpha^2}} e^{-2i\pi fu} du. \quad (\text{S-12})$$

It can be calculated by first reorganizing the quadratic terms of the exponential

$$\begin{aligned} Q &= \frac{1}{\tau^2}(u - t_0)^2 + \frac{1}{\alpha^2}(u - t)^2 \\ &= \left(\frac{1}{\tau^2} + \frac{1}{\alpha^2}\right)u^2 - 2u\left(\frac{t_0}{\tau^2} + \frac{t}{\alpha^2}\right) + \frac{t_0^2}{\tau^2} + \frac{t^2}{\alpha^2}. \end{aligned}$$

Setting

$$\hat{t} = \frac{\frac{t_0}{\tau^2} + \frac{t}{\alpha^2}}{\frac{1}{\tau^2} + \frac{1}{\alpha^2}},$$

we obtain

$$Q = \left(\frac{1}{\tau^2} + \frac{1}{\alpha^2}\right)(u - \hat{t})^2 + \frac{t_0^2}{\tau^2} + \frac{t^2}{\alpha^2} - \left(\frac{1}{\tau^2} + \frac{1}{\alpha^2}\right)\hat{t}^2.$$

The term that does not depend on  $u$  can be expanded and simplified to yield

$$\begin{aligned} \frac{t_0^2}{\tau^2} + \frac{t^2}{\alpha^2} - \left(\frac{1}{\tau^2} + \frac{1}{\alpha^2}\right)\hat{t}^2 &= \frac{\frac{1}{\tau^2}\frac{1}{\alpha^2}}{\frac{1}{\tau^2} + \frac{1}{\alpha^2}}(t - t_0)^2 \\ &= \frac{1}{\tau^2 + \alpha^2}(t - t_0)^2, \end{aligned}$$

so that

$$Q = \left(\frac{1}{\tau^2} + \frac{1}{\alpha^2}\right)(u - \hat{t})^2 + \frac{(t - t_0)^2}{\tau^2 + \alpha^2}$$

and

$$I_3(t, \alpha, t_0, f) = e^{\frac{(t-t_0)^2}{2(\tau^2+\alpha^2)}} \frac{1}{\sqrt{2\pi\alpha^2}} \int \Omega \cos(2\pi\nu u + \phi) e^{-\frac{1}{2}\left(\frac{1}{\tau^2} + \frac{1}{\alpha^2}\right)(u-\hat{t})^2} e^{-2i\pi f u} du. \quad (\text{S-13})$$

Setting

$$\beta = \frac{1}{\tau^2} + \frac{1}{\alpha^2}, \quad (\text{S-14})$$

we can then applying (S-10):

$$\begin{aligned} I_3(t, \alpha, t_0, f) &= \frac{\beta}{\alpha} e^{\frac{(t-t_0)^2}{2(\tau^2+\alpha^2)}} \frac{1}{\sqrt{2\pi\beta^2}} \int \Omega \cos(2\pi\nu u + \phi) e^{-\frac{(u-\hat{t})^2}{2\beta^2}} e^{-2i\pi f u} du \\ &= \frac{\beta}{\alpha} e^{\frac{(t-t_0)^2}{2(\tau^2+\alpha^2)}} I_2(\Omega, \hat{t}, \beta, f) \\ &= \frac{\beta}{\alpha} e^{-\frac{(t-t_0)^2}{2(\tau^2+\alpha^2)}} \left\{ \frac{\Omega}{2} e^{-\frac{1}{2}(2\pi\beta)^2(f-\nu)^2} e^{i[\phi-2\pi(f-\nu)\hat{t}]} + \frac{\Omega}{2} e^{-\frac{1}{2}(2\pi\beta)^2(f+\nu)^2} e^{i[-\phi-2\pi(f-\nu)\hat{t}]} \right\}. \end{aligned} \quad (\text{S-15})$$

Note that, for  $\tau^2 \ll \alpha^2$ , we have  $\beta^2 \approx \tau^2$ , whereas  $\beta^2 \approx \alpha^2$  for  $\tau^2 \gg \alpha^2$ .

## 2.2 S-transform of oscillatory signal

We here calculate the time-frequency transform of a signal of the form given by Equation (24) of the manuscript. Application of (S-10) with  $\alpha = 1/f$  yields

$$\begin{aligned} T_x(t, f) &= \frac{|f|}{\sqrt{2\pi}} \int \Omega \cos(2\pi\nu u + \phi) e^{-\frac{f^2(u-t)^2}{2}} e^{-2i\pi f u} du \\ &= \frac{\Omega}{2} e^{-\frac{1}{2}(2\pi)^2\left(1-\frac{\nu}{f}\right)^2} e^{i[\phi-2\pi(f-\nu)t]} + \frac{\Omega}{2} e^{-\frac{1}{2}(2\pi)^2\left(1+\frac{\nu}{f}\right)^2} e^{i[-\phi-2\pi(f-f_0)t]}. \end{aligned} \quad (\text{S-16})$$

## 2.3 Approximation

### 2.3.1 General approach

We here provide an approximation for the modulus and argument of  $T_x(t, f)$  in (S-16). We first express  $T_x(t, f)$  as

$$T_x(t, f) = \frac{\Omega}{2} e^{-\frac{1}{2}(2\pi)^2 \left(1 - \frac{\nu}{f}\right)^2} e^{i[\phi - 2\pi(f - \nu)t]} \left[ 1 + e^{-8\pi^2 \frac{\nu}{f}} e^{i(-2\phi - 4\pi\nu t)} \right].$$

Setting

$$T_x^\dagger(t, f) = \frac{\Omega}{2} e^{-\frac{1}{2}(2\pi)^2 \left(1 - \frac{\nu}{f}\right)^2} e^{i[\phi - 2\pi(f - \nu)t]} \quad (\text{S-17})$$

and

$$\epsilon(t, f) = e^{-8\pi^2 \frac{\nu}{f}} e^{i(-2\phi - 4\pi\nu t)}, \quad (\text{S-18})$$

we can express  $T_x(t, f)$  as

$$T_x(t, f) = T_x^\dagger(t, f) [1 + \epsilon(t, f)]. \quad (\text{S-19})$$

From there, the module and argument of  $T_x(t, f)$  can be calculated as

$$|T_x(t, f)| = |T_x^\dagger(t, f)| |1 + \epsilon(t, f)| \quad (\text{S-20})$$

$$\arg[T_x(t, f)] = \arg[T_x^\dagger(t, f)] + \arg[1 + \epsilon(t, f)]. \quad (\text{S-21})$$

The module and argument of  $T_x^\dagger(t, f)$  can be easily calculated, yielding

$$|T_x^\dagger(t, f)| = \frac{\Omega}{2} e^{-\frac{1}{2}(2\pi)^2 \left(1 - \frac{\nu}{f}\right)^2} \quad (\text{S-22})$$

$$\arg[T_x^\dagger(t, f)] = \phi - 2\pi(f - \nu)t. \quad (\text{S-23})$$

The module and argument of  $1 + \epsilon(t, f)$  are not quite as straightforward to obtain. See Figure 1 for a schematic description. Since we only consider  $f > 0$ , we have  $e^{-8\pi^2 \frac{\nu}{f}} < 1$ , so that  $0 < \epsilon(t, f) < 1$  and  $1 + \epsilon(t, f)$  has modulus in  $]0, 2[$  and argument in  $] -\frac{\pi}{2}, \frac{\pi}{2}[$ . We define  $\epsilon_m(t, f)$  and  $\epsilon_a(t, f)$  as

$$|1 + \epsilon(t, f)| = 1 + \epsilon_m(t, f) \quad (\text{S-24})$$

$$\arg[1 + \epsilon(t, f)] = \epsilon_a(t, f). \quad (\text{S-25})$$

We now provide bounds for both quantities.

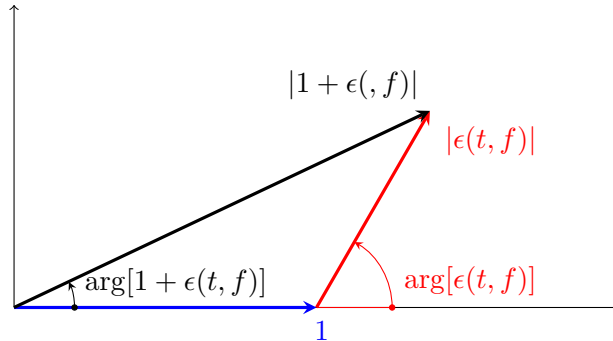

Figure 1: **Modulus and argument of  $1 + \epsilon(t, f)$ .**

### 2.3.2 Bounds for $\epsilon_m(t, f)$

From (S-24) and (S-18), we have

$$\begin{aligned}
[1 + \epsilon_m(t, f)]^2 &= |1 + \epsilon(t, f)|^2 \\
&= \left| 1 + e^{-8\pi^2 \frac{\nu}{f}} e^{i(-2\phi - 4\pi\nu t)} \right|^2 \\
&= \left[ 1 + e^{-8\pi^2 \frac{\nu}{f}} \cos(2\phi + 4\pi\nu t) \right]^2 \\
&\quad + \left[ e^{-8\pi^2 \frac{\nu}{f}} \sin(2\phi + 4\pi\nu t) \right]^2 \\
&= 1 + 2e^{-8\pi^2 \frac{\nu}{f}} \cos(2\phi + 4\pi\nu t) \\
&\quad + e^{-16\pi^2 \frac{\nu}{f}},
\end{aligned}$$

so that

$$\begin{aligned}
[1 + \epsilon_m(t, f)]^2 &< 1 + 2e^{-8\pi^2 \frac{\nu}{f}} + e^{-16\pi^2 \frac{\nu}{f}} \\
&< \left( 1 + e^{-8\pi^2 \frac{\nu}{f}} \right)^2 \\
1 + \epsilon_m(t, f) &< 1 + e^{-8\pi^2 \frac{\nu}{f}}
\end{aligned} \tag{S-26}$$

and

$$\begin{aligned}
[1 + \epsilon_m(t, f)]^2 &> 1 - 2e^{-8\pi^2 \frac{\nu}{f}} + e^{-16\pi^2 \frac{\nu}{f}} \\
&> \left( 1 - e^{-8\pi^2 \frac{\nu}{f}} \right)^2 \\
1 + \epsilon_m(t, f) &> 1 - e^{-8\pi^2 \frac{\nu}{f}}.
\end{aligned} \tag{S-27}$$

From (S-26) and (S-27), we are led to

$$|\epsilon_m(t, f)| < e^{-8\pi^2 \frac{\nu}{f}}. \tag{S-28}$$

Numerically, we have for  $f < f_0 = 10\nu$

$$|\epsilon_m(t, f)| < e^{-8\pi^2 \frac{\nu}{f}} < e^{-8\pi^2 \frac{\nu}{f_0}} \approx 3.8 \times 10^{-4}. \tag{S-29}$$

### 2.3.3 Bounds for $\epsilon_a(t, f)$

Since  $\epsilon_a(t, f)$  is in  $]-\frac{\pi}{2}, \frac{\pi}{2}[$ , its argument can be expressed from (S-25) and (S-18) in terms of the tangent function, yielding

$$\tan[\epsilon_a(t, f)] = \frac{e^{-8\pi^2 \frac{\nu}{f}} \sin(2\phi + 4\pi\nu t)}{1 + e^{-8\pi^2 \frac{\nu}{f}} \cos(2\phi + 4\pi\nu t)}.$$

The variations of the right-hand side of the expression as a function of  $t$  can be investigated (see §1.1 of Supplementary Material #3), showing that

$$|\tan[\epsilon_a(t, f)]| \leq \frac{e^{-8\pi^2 \frac{\nu}{f}}}{\sqrt{1 - e^{-16\pi^2 \frac{\nu}{f}}}},$$

or, equivalently,

$$|\epsilon_a(t, f)| < \arctan \left[ \frac{e^{-8\pi^2 \frac{\nu}{f}}}{\sqrt{1 - e^{-16\pi^2 \frac{\nu}{f}}}} \right]. \tag{S-30}$$

Since the upper bound is an increasing function of  $f$  (see §1.2 of Supplementary Material #3), we obtain in particular that, for  $f < f_0$ ,

$$|\epsilon_a(t, f)| < \arctan \left[ \frac{e^{-8\pi^2 \frac{\nu}{f_0}}}{\sqrt{1 - e^{-16\pi^2 \frac{\nu}{f_0}}}} \right] \approx 3.8 \times 10^{-4}. \tag{S-31}$$

### 2.3.4 Modulus of $T_x(t, f)$

According to (S-20), (S-22), and (S-24), the modulus of  $T_x(t, f)$  is given by

$$|T_x(t, f)| = \frac{\Omega}{2} e^{-\frac{1}{2}(2\pi)^2 \left(1 - \frac{\nu}{f}\right)^2} [1 + \epsilon_m(t, f)], \quad (\text{S-32})$$

with, according to (S-28),

$$|\epsilon_m(t, f)| < 1 \quad (\text{S-33})$$

and, using (S-29) for  $f < 10\nu$ ,

$$|\epsilon_m(t, f)| < 3.8 \times 10^{-4}. \quad (\text{S-34})$$

Note that, for  $f \geq 10\nu$ , we have

$$|T_x^\dagger(t, f)| < 1.1 \times 10^{-7} \frac{\Omega}{2}, \quad (\text{S-35})$$

which, together with (S-20) the fact that  $\epsilon_m(t, f) \in ]0, 2[$ , yields the following upper bound

$$|T_x(t, f)| < 2.2 \times 10^{-7} \frac{\Omega}{2}. \quad (\text{S-36})$$

As a consequence, values of modulus are not relevant for  $f \geq 10\nu$ .

### 2.3.5 Argument of $T_x(t, f)$

According to (S-21), (S-23), and (S-25), the argument of  $T_x(t, f)$  is given by

$$\arg [T_x(t, f)] = \phi - 2\pi(f - \nu)t + \epsilon_a(t, f), \quad (\text{S-37})$$

with, according to (S-30)

$$|\epsilon_a(t, f)| < \arctan \left[ \frac{e^{-8\pi^2 \frac{\nu}{f}}}{\sqrt{1 - e^{-16\pi^2 \frac{\nu}{f}}}} \right]$$

and, using (S-31) for  $f \geq 10\nu$ ,

$$|\epsilon_a(t, f)| < 3.8 \times 10^{-4}. \quad (\text{S-38})$$

### 2.3.6 Summary of bounds

Since we are interested in  $f > 0$ , we always have  $|\epsilon(t, f)| < 1$ . Furthermore, for  $f < f_0 = 10\nu$ ,  $|\epsilon(t, f)| < 3.8 \times 10^{-4}$ . For  $f \geq 10\nu$ ,  $|\epsilon(t, f)|$  can be larger (up to the upper bound of 1, reached for  $f \rightarrow \infty$ ), but  $T_x^\dagger(t, f)$  itself is then negligible, as  $|T_x^\dagger(t, f)| < 1.1 \times 10^{-7} \Omega/2$ .

For the amplitude,  $|\epsilon_m(t, f)| < e^{-8\pi^2 \frac{\nu}{f}}$  and, for  $f < f_0$ ,  $|\epsilon_m(t, f)| < 3.8 \times 10^{-4}$ . For the phase,  $|\tan \epsilon_a(t, f)| < e^{-8\pi^2 \frac{\nu}{f}} / \sqrt{1 - e^{-16\pi^2 \frac{\nu}{f}}}$  and, for  $f < f_0$ ,  $|\epsilon_a(t, f)| < 3.8 \times 10^{-4}$ .

## 2.4 Model with varying amplitude and phase

To derive an asymptotic form for  $E(\text{POWavg}^\dagger)$ , we first need to calculate the expectation of the time-frequency transform. Using Equation (46) of the manuscript, we obtain

$$\begin{aligned} E \left[ T_{x_n}^\dagger(t, f) \right] &= \frac{1}{2} e^{-\frac{1}{2}(2\pi)^2 \left(1 - \frac{\nu_0}{f}\right)^2} e^{-2i\pi(f - \nu_0)t} E \left( \Omega_n e^{i\phi_n} \right) \\ &= \frac{1}{2} e^{-\frac{1}{2}(2\pi)^2 \left(1 - \frac{\nu_0}{f}\right)^2} e^{-2i\pi(f - \nu_0)t} E(\Omega_n) E(e^{i\phi_n}) \\ &= \frac{\Omega_0 \rho}{2} e^{-\frac{1}{2}(2\pi)^2 \left(1 - \frac{\nu_0}{f}\right)^2} e^{i[\phi_0 - 2\pi(f - \nu_0)t]}, \end{aligned}$$

whose power is given by

$$\left| E \left[ T_{x_n}^\dagger(t, f) \right] \right|^2 = \left[ \frac{\Omega_0 \rho}{2} e^{-\frac{1}{2}(2\pi)^2 \left(1 - \frac{\nu_0}{f}\right)^2} \right]^2. \quad (\text{S-39})$$

Equation (23) of the manuscript then implies

$$\mathbb{E} \left( \text{POWav}^\dagger \right) = \left[ \frac{\Omega_0 \rho}{2} e^{-\frac{1}{2}(2\pi)^2 \left(1 - \frac{\nu_0}{f}\right)^2} \right]^2 + O \left( \frac{1}{N} \right). \quad (\text{S-40})$$

## 2.5 Model with varying amplitude, frequency, and phase

### 2.5.1 Preliminary results

We first provide the expectation of three quantities:

$$E_1(t, f) = \mathbb{E} \left[ e^{-2i\pi(f-\nu)t} \right] \quad (\text{S-41})$$

$$E_2(\alpha, f) = \mathbb{E} \left[ e^{-\frac{1}{2}(2\pi\alpha)^2(f-\nu)^2} \right] \quad (\text{S-42})$$

$$E_3(t, \alpha, f) = \mathbb{E} \left[ e^{-\frac{1}{2}(2\pi\alpha)^2(f-\nu)^2 - 2i\pi(f-\nu)t} \right], \quad (\text{S-43})$$

when  $\nu$  is normally distributed with mean  $\nu_0$  and variance  $\tau_\nu^2$ .

**Calculation of  $E_1(t, f)$ .** The first quantity is given by

$$\begin{aligned} E_1(t, f) &= \frac{1}{\sqrt{2\pi\tau_\nu^2}} \int_{-\infty}^{+\infty} e^{-2i\pi(f-\nu)t} e^{-\frac{1}{2\tau_\nu^2}(\nu-\nu_0)^2} d\nu \\ &= \frac{1}{\sqrt{2\pi\tau_\nu^2}} e^{-2i\pi ft} \int_{-\infty}^{+\infty} e^{2i\pi\nu t} e^{-\frac{1}{2\tau_\nu^2}(\nu-\nu_0)^2} d\nu \\ &= \frac{1}{\sqrt{2\pi\tau_\nu^2}} e^{-2i\pi ft} \int_{-\infty}^{+\infty} e^{-2i\pi\nu(-t)} e^{-\frac{1}{2\tau_\nu^2}(\nu-\nu_0)^2} d\nu \\ &= e^{-2i\pi ft} I_1(\nu_0, \tau_\nu, -t) \\ &= e^{-2i\pi ft} e^{-\frac{1}{2}(2\pi\tau_\nu t)^2} e^{2i\pi\nu_0 t} \\ &= e^{-\frac{1}{2}(2\pi\tau_\nu t)^2} e^{-2i\pi(f-\nu_0)t}, \end{aligned}$$

where  $I_1$  is defined in (S-7).

**Calculation of  $E_2(\alpha, f)$ .** The second quantity is given by

$$E_2(\alpha, f) = \frac{1}{\sqrt{2\pi\tau_\nu^2}} \int_{-\infty}^{+\infty} e^{-\frac{1}{2}(2\pi\alpha)^2(f-\nu)^2} e^{-\frac{1}{2\tau_\nu^2}(\nu-\nu_0)^2} d\nu.$$

We reorganize the quadratic terms in the exponential

$$\begin{aligned} Q &= (2\pi\alpha)^2(f-\nu)^2 + \frac{1}{\tau_\nu^2}(\nu-\nu_0)^2 \\ &= \left[ (2\pi\alpha)^2 + \frac{1}{\tau_\nu^2} \right] \nu^2 - 2\nu \left[ (2\pi\alpha)^2 f + \frac{\nu_0}{\tau_\nu^2} \right] \\ &\quad + (2\pi\alpha)^2 f^2 + \frac{\nu_0^2}{\tau_\nu^2}. \end{aligned}$$

Setting

$$\hat{\nu} = \frac{(2\pi\alpha)^2 f + \frac{\nu_0}{\tau_\nu^2}}{(2\pi\alpha)^2 + \frac{1}{\tau_\nu^2}},$$

we obtain

$$Q = \left[ (2\pi\alpha)^2 + \frac{1}{\tau_\nu^2} \right] (\nu - \nu_0)^2 + (2\pi\alpha)^2 f^2 + \frac{\nu_0^2}{\tau_\nu^2} - \left[ (2\pi\alpha)^2 + \frac{1}{\tau_\nu^2} \right] \hat{\nu}^2.$$

The term that does not depend on  $\nu$  can be expanded and simplified to yield

$$\begin{aligned} (2\pi\alpha)^2 f^2 + \frac{\nu_0^2}{\tau_\nu^2} - \left[ (2\pi\alpha)^2 + \frac{1}{\tau_\nu^2} \right] \hat{\nu}^2 &= \frac{(2\pi\alpha)^2 \frac{1}{\tau_\nu^2}}{(2\pi\alpha)^2 + \frac{1}{\tau_\nu^2}} (f - \nu_0)^2 \\ &= \frac{(2\pi\alpha)^2}{(2\pi\alpha)^2 \tau_\nu^2 + 1} (f - \nu_0)^2, \end{aligned}$$

so that

$$Q = \left[ (2\pi\alpha)^2 + \frac{1}{\tau_\nu^2} \right] (\nu - \nu_0)^2 + \frac{(2\pi\alpha)^2}{(2\pi\alpha)^2 \tau_\nu^2 + 1} (f - \nu_0)^2$$

and

$$E_2(\alpha, f) = \frac{1}{\sqrt{2\pi\tau_\nu^2}} e^{-\frac{1}{2} \frac{(2\pi\alpha)^2}{(2\pi\alpha)^2 \tau_\nu^2 + 1} (f - \nu_0)^2} \int_{-\infty}^{+\infty} e^{-\frac{1}{2} \left[ (2\pi\alpha)^2 + \frac{1}{\tau_\nu^2} \right] (\nu - \nu_0)^2} d\nu. \quad (\text{S-44})$$

The integral can be calculated using the fact that a normal distribution sums to 1 (Polyanin and Manzhirov, 2007, Equation (20.2.4.5)), leading to

$$\int_{-\infty}^{+\infty} e^{-\frac{1}{2} \left[ (2\pi\alpha)^2 + \frac{1}{\tau_\nu^2} \right] (\nu - \nu_0)^2} d\nu = \sqrt{\frac{2\pi}{(2\pi\alpha)^2 + \frac{1}{\tau_\nu^2}}}$$

and

$$E_2(\alpha, f) = \frac{1}{\sqrt{(2\pi\alpha)^2 \tau_\nu^2 + 1}} e^{-\frac{1}{2} \frac{(2\pi\alpha)^2}{(2\pi\alpha)^2 \tau_\nu^2 + 1} (f - \nu_0)^2}.$$

**Calculation of  $E_3(t, \alpha, f)$ .**  $E_3(t, \alpha, f)$  is given by

$$E_3(t, \alpha, f) = \frac{1}{\sqrt{2\pi\tau_\nu^2}} \int_{-\infty}^{+\infty} e^{-\frac{1}{2} (2\pi\alpha)^2 (f - \nu)^2} e^{-\frac{1}{2\tau_\nu^2} (\nu - \nu_0)^2} e^{-2i\pi(f - \nu)t} d\nu.$$

We use (S-44) to express the real term in the exponential, yielding

$$E_3(t, \alpha, f) = \frac{1}{\sqrt{2\pi\tau_\nu^2}} e^{-\frac{1}{2} \frac{(2\pi\alpha)^2}{(2\pi\alpha)^2 \tau_\nu^2 + 1} (f - \nu_0)^2} \int_{-\infty}^{+\infty} e^{-\frac{1}{2} \left[ (2\pi\alpha)^2 + \frac{1}{\tau_\nu^2} \right] (\nu - \nu_0)^2} e^{-2i\pi(f - \nu)t} d\nu.$$

The integral in this expression rereads

$$\int_{-\infty}^{+\infty} e^{-\frac{1}{2} \left[ (2\pi\alpha)^2 + \frac{1}{\tau_\nu^2} \right] (\nu - \nu_0)^2} e^{-2i\pi(f - \nu)t} d\nu = e^{-2i\pi f t} \int_{-\infty}^{+\infty} e^{-\frac{1}{2} \left[ (2\pi\alpha)^2 + \frac{1}{\tau_\nu^2} \right] (\nu - \nu_0)^2} e^{2i\pi \nu t} d\nu.$$

Performing the parameter change  $\xi = -\nu$ , we obtain

$$\int_{-\infty}^{+\infty} e^{-\frac{1}{2} \left[ (2\pi\alpha)^2 + \frac{1}{\tau_\nu^2} \right] (\nu - \nu_0)^2} e^{2i\pi \nu t} d\nu = \int_{-\infty}^{+\infty} e^{-\frac{1}{2} \left[ (2\pi\alpha)^2 + \frac{1}{\tau_\nu^2} \right] (\xi + \nu_0)^2} e^{-2i\pi \xi t} d\xi.$$

This integral can be calculated using (S-8), leading to

$$\int_{-\infty}^{+\infty} e^{-\frac{1}{2} \left[ (2\pi\alpha)^2 + \frac{1}{\tau_\nu^2} \right] (\xi + \nu_0)^2} e^{-2i\pi \xi t} d\xi = \sqrt{\frac{2\pi\tau_\nu^2}{(2\pi\alpha)^2 \tau_\nu^2 + 1}} e^{-\frac{1}{2} \frac{(2\pi t)^2}{(2\pi\alpha)^2 + \frac{1}{\tau_\nu^2}}} e^{2i\pi \nu_0 t}.$$

We therefore have

$$\int_{-\infty}^{+\infty} e^{-\frac{1}{2} \left[ (2\pi\alpha)^2 + \frac{1}{\tau_\nu^2} \right] (\nu - \nu_0)^2} e^{-2i\pi(f - \nu)t} d\nu = \sqrt{\frac{2\pi\tau_\nu^2}{(2\pi\alpha)^2 \tau_\nu^2 + 1}} e^{-\frac{1}{2} \frac{(2\pi t)^2}{(2\pi\alpha)^2 + \frac{1}{\tau_\nu^2}}} e^{-2i\pi(f - \nu_0)t}$$

and

$$\begin{aligned} E_3(t, \alpha, f) &= \frac{1}{\sqrt{(2\pi\alpha)^2 \tau_\nu^2 + 1}} e^{-\frac{1}{2} \frac{(2\pi\alpha)^2}{(2\pi\alpha)^2 \tau_\nu^2 + 1} (f - \nu_0)^2} e^{-\frac{1}{2} \frac{(2\pi t)^2}{(2\pi\alpha)^2 + \frac{1}{\tau_\nu^2}}} e^{-2i\pi(f - \nu_0)t} \\ &= \frac{1}{\sqrt{(2\pi\alpha)^2 \tau_\nu^2 + 1}} e^{-2i\pi(f - \nu_0)t} e^{-\frac{1}{2} \frac{(2\pi\alpha)^2}{(2\pi\alpha)^2 \tau_\nu^2 + 1} \left[ (f - \nu_0)^2 + \left( \frac{\tau_\nu}{\alpha} \right)^2 t^2 \right]}. \end{aligned}$$

### 2.5.2 Expectation of $|T_x^\dagger(t, f)|$

With the definition of  $T_x^\dagger(t, f)$  from Equation (28) from the manuscript, we obtain that

$$\begin{aligned} \mathbb{E} \left[ |T_x^\dagger(t, f)| \right] &= \mathbb{E} \left[ \frac{\Omega}{2} e^{-\frac{1}{2}(2\pi)^2 \left(1 - \frac{\nu}{f}\right)^2} \right] \\ &= \mathbb{E} \left[ \frac{\Omega}{2} \right] \mathbb{E} \left[ e^{-\frac{1}{2}(2\pi)^2 \left(1 - \frac{\nu}{f}\right)^2} \right], \end{aligned}$$

since  $\Omega$  and  $\nu$  are independent. The first expectation in the right-hand is straightforward to calculate, yielding

$$\mathbb{E} \left[ \frac{\Omega}{2} \right] = \frac{\Omega_0}{2}. \quad (\text{S-45})$$

The second expectation in the right-hand side needs to be calculated explicitly as

$$\begin{aligned} \mathbb{E} \left[ e^{-\frac{1}{2}(2\pi)^2 \left(1 - \frac{\nu}{f}\right)^2} \right] &= \int e^{-\frac{1}{2}(2\pi)^2 \left(1 - \frac{\nu}{f}\right)^2} p(\nu) d\nu \\ &= \frac{1}{\sqrt{2\pi\tau_\nu^2}} \int e^{-\frac{1}{2}(2\pi)^2 \left(1 - \frac{\nu}{f}\right)^2} e^{-\frac{1}{2\tau_\nu^2}(\nu - \nu_0)^2} d\nu \\ &= E_2 \left( \frac{1}{f}, f \right) \\ &= \frac{1}{\sqrt{\left(\frac{2\pi\tau_\nu^2}{f}\right)^2 + 1}} e^{-\frac{1}{2} \frac{(2\pi)^2}{\left(\frac{2\pi\tau_\nu^2}{f}\right)^2 + 1} \left(1 - \frac{\nu_0}{f}\right)^2}. \end{aligned} \quad (\text{S-46})$$

### 2.5.3 Expectation of $e^{i \arg[T_x^\dagger(t, f)]}$

We have

$$\begin{aligned} \mathbb{E} \left\{ e^{i \arg[T_x^\dagger(t, f)]} \right\} &= \mathbb{E} \left\{ e^{i[\phi - 2\pi(f - \nu)t]} \right\} \\ &= \mathbb{E} \left( e^{i\phi} \right) \mathbb{E} \left[ e^{-2i\pi(f - \nu)t} \right], \end{aligned} \quad (\text{S-47})$$

since  $\phi$  and  $\nu$  are independent. According to Equation (35) of the manuscript, the value of the first expectation of the right-hand side is given by  $\rho e^{i\phi_0}$ . As to the second expectation, it yields

$$\begin{aligned} \mathbb{E} \left[ e^{-2i\pi(f - \nu)t} \right] &= E_1(t, f) \\ &= e^{-\frac{1}{2}(2\pi\tau_\nu t)^2} e^{-2i\pi(f - \nu_0)t}. \end{aligned} \quad (\text{S-48})$$

### 2.5.4 Expectation of $T_x^\dagger(t, f)$

We have

$$\begin{aligned} \mathbb{E} \left[ T_x^\dagger(t, f) \right] &= \mathbb{E} \left\{ \frac{\Omega}{2} e^{-\frac{1}{2}(2\pi)^2 \left(1 - \frac{\nu}{f}\right)^2} e^{i[\phi - 2\pi(f - \nu)t]} \right\} \\ &= \mathbb{E} \left( \frac{\Omega}{2} \right) \mathbb{E} \left( e^{i\phi} \right) \mathbb{E} \left[ e^{-\frac{1}{2}(2\pi)^2 \left(1 - \frac{\nu}{f}\right)^2 - 2i\pi(f - \nu)t} \right], \end{aligned} \quad (\text{S-49})$$

with  $E(\Omega/2) = \Omega_0/2$ ,  $E(e^{i\phi}) = \rho e^{i\phi_0}$ , and

$$\begin{aligned} E \left[ e^{-\frac{1}{2}(2\pi)^2 \left(1 - \frac{\nu}{f}\right)^2 - 2i\pi(f-\nu)t} \right] &= E_3 \left( t, \frac{1}{f}, f \right) \\ &= \frac{1}{\sqrt{\left(\frac{2\pi\tau_\nu}{f}\right)^2 + 1}} e^{-2i\pi(f-\nu_0)t} e^{-\frac{1}{2} \frac{(2\pi)^2}{\left(\frac{2\pi\tau_\nu}{f}\right)^2 + 1} \left[ \left(1 - \frac{\nu_0}{f}\right)^2 + \tau_\nu^2 t^2 \right]}. \end{aligned} \quad (\text{S-50})$$

## 2.6 Summary of results

The results regarding the S-transform of an oscillatory model of increasing complexity are summarized here.

| Model                                 | Section | Distributions                                                                                                                                                              | Relationship between quantities                                                      |
|---------------------------------------|---------|----------------------------------------------------------------------------------------------------------------------------------------------------------------------------|--------------------------------------------------------------------------------------|
| varying $\phi$                        | §II-D4  | $\begin{cases} \phi_n \sim \text{VonMises}(\phi_0, \kappa) \\ \Omega_n = \Omega_0 \\ \nu_n = \nu_0 \end{cases}$                                                            | $\text{POWavg} = \text{avgAMP}^2 \times \text{ITC}^2$                                |
| varying $\phi$ and $\Omega$           | §II-D5  | $\begin{cases} \phi_n \sim \text{VonMises}(\phi_0, \kappa) \\ \Omega_n \sim \mathcal{N}(\Omega_0, \tau_\Omega^2) \\ \nu_n = \nu_0 \end{cases}$                             | $E[\text{POWavg} - \text{avgAMP}^2 \times \text{ITC}^2] = O\left(\frac{1}{N}\right)$ |
| varying $\phi$ , $\Omega$ , and $\nu$ | §II-D6  | $\begin{cases} \phi_n \sim \text{VonMises}(\phi_0, \kappa) \\ \Omega_n \sim \mathcal{N}(\Omega_0, \tau_\Omega^2) \\ \nu_n \sim \mathcal{N}(\nu_0, \tau_\nu^2) \end{cases}$ | Nontrivial, see Equation (70)                                                        |

## 3 Proof of general relationship between avgAMP, ITC, and POWavg

We here provide a sketch of proof. Detailed results can be found in [§2 of Supplementary Material #3](#). We expand  $\text{avgAMP}^2 \times \text{ITC}^2$  from (S-1) and (S-3), yielding

$$\begin{aligned} \text{avgAMP}_{x_{1:N}}(t, f)^2 \times \text{ITC}_{x_{1:N}}(t, f)^2 &= \underbrace{\frac{1}{N^3} \sum_{k=1}^N |T_{x_k}(t, f)|^2}_{S_1} + \underbrace{\frac{1}{N^3} \sum_{k \neq l} |T_{x_k}(t, f)| |T_{x_l}(t, f)|}_{S_2} \\ &\quad + \underbrace{\frac{1}{N^4} \left\{ \sum_{m \neq n} e^{i[\theta_{x_m}(t, f) - \theta_{x_n}(t, f)]} \right\} \left[ \sum_{k=1}^N |T_{x_k}(t, f)|^2 \right]}_{P_1} \\ &\quad + \underbrace{\frac{1}{N^4} \left\{ \sum_{m \neq n} e^{i[\theta_{x_m}(t, f) - \theta_{x_n}(t, f)]} \right\} \times \left[ \sum_{k \neq l} |T_{x_k}(t, f)| |T_{x_l}(t, f)| \right]}_{P_2}. \end{aligned} \quad (\text{S-51})$$

$P_1$  of (S-51) can be further expanded, yielding

$$\begin{aligned}
P_1 = & \underbrace{\frac{1}{N^4} \sum_{m \neq n} |T_{x_m}(t, f)|^2 e^{i[\theta_{x_m}(t, f) - \theta_{x_n}(t, f)]}}_{S_3} \\
& + \underbrace{\frac{1}{N^4} \sum_{m \neq n} |T_{x_n}(t, f)|^2 e^{i[\theta_{x_m}(t, f) - \theta_{x_n}(t, f)]}}_{S_4} \\
& + \underbrace{\frac{1}{N^4} \sum_{m \neq n} e^{i[\theta_{x_m}(t, f) - \theta_{x_n}(t, f)]} \sum_{k \notin \{m, n\}} |T_{x_k}(t, f)|^2}_{S_5}.
\end{aligned} \tag{S-52}$$

$P_2$  of (S-51) can also be expanded:

$$\begin{aligned}
P_2 = & \underbrace{\frac{2}{N^4} \sum_{m \neq n} |T_{x_m}(t, f)| |T_{x_n}(t, f)| e^{i[\theta_{x_m}(t, f) - \theta_{x_n}(t, f)]}}_{S_6} \\
& + \underbrace{\frac{2}{N^4} \sum_{m \neq n} |T_{x_m}(t, f)| e^{i[\theta_{x_m}(t, f) - \theta_{x_n}(t, f)]} \sum_{l \notin \{m, n\}} |T_{x_l}(t, f)|}_{S_7} \\
& + \underbrace{\frac{2}{N^4} \sum_{m \neq n} |T_{x_n}(t, f)| e^{i[\theta_{x_m}(t, f) - \theta_{x_n}(t, f)]} \sum_{l \notin \{m, n\}} |T_{x_l}(t, f)|}_{S_8} \\
& + \underbrace{\frac{1}{N^4} \sum_{m \neq n} e^{i[\theta_{x_m}(t, f) - \theta_{x_n}(t, f)]} \sum_{l \notin \{m, n\}} |T_{x_l}(t, f)| \sum_{k \notin \{l, m, n\}} |T_{x_k}(t, f)|}_{S_9}.
\end{aligned} \tag{S-53}$$

We were able to expand  $\text{avgAMP}_{x_{1:N}}(t, f)^2 \times \text{ITC}_{x_{1:N}}(t, f)^2$  into 9 terms: two ( $S_1$  and  $S_2$ ) from (S-51), three ( $S_3$  to  $S_5$ ) from (S-52), and 4 ( $S_6$  to  $S_9$ ) from (S-53). We can now calculate the expectation of  $\text{avgAMP}_{x_{1:N}}(t, f)^2 \times \text{ITC}_{x_{1:N}}(t, f)^2$  term by term.

$$E(S_1) = \frac{1}{N^2} E[|T_x(t, f)|^2],$$

for a global contribution that is  $O(1/N^2)$ ;

$$E(S_2) = \frac{N-1}{N^2} E[|T_x(t, f)|^2],$$

for a global contribution that is  $O(1/N)$ ;

$$E(S_3) = \frac{N-1}{N^3} E[|T_x(t, f)|^2 e^{i\theta_x(t, f)}] E[e^{i\theta_x(t, f)}]^*,$$

which is  $O(1/N^2)$ ;

$$E(S_4) = \frac{N-1}{N^3} E[|T_x(t, f)|^2 e^{-i\theta_x(t, f)}] E[e^{i\theta_x(t, f)}],$$

which is also  $O(1/N^2)$ ;

$$E(S_5) = \frac{(N-1)(N-2)}{N^3} E \left[ |T_x(t, f)|^2 \right] \left| E \left[ e^{i\theta_x(t, f)} \right] \right|^2,$$

which is  $O(1/N)$ ;

$$E(S_6) = \frac{2(N-1)}{N^3} |E[T_x(t, f)]|^2,$$

which is  $O(1/N^2)$ ;

$$E(S_7) = \frac{2(N-1)(N-2)}{N^3} E[T_x(t, f)] E \left[ e^{i\theta_x(t, f)} \right]^* E[|T_x(t, f)|],$$

which is  $O(1/N)$ ;

$$E(S_8) = \frac{2(N-1)(N-2)}{N^3} E[T_x(t, f)]^* E \left[ e^{i\theta_x(t, f)} \right] E[|T_x(t, f)|],$$

which is  $O(1/N)$ ;

$$E(S_9) = \frac{(N-1)(N-2)(N-3)}{N^3} \left| E \left[ e^{i\theta_x(t, f)} \right] \right|^2 E[|T_x(t, f)|]^2,$$

which is the only term to be  $O(1)$ . Putting all expressions together, we are led to

$$E(\text{avgAMP}^2 \times \text{ITC}^2) = \left| E \left[ e^{i\theta_x(t, f)} \right] \right|^2 E[|T_x(t, f)|]^2 + O\left(\frac{1}{N}\right). \quad (\text{S-54})$$

We now need to express POWavg. From (S-6), we have

$$E[\text{POWavg}_{x_{1:N}}(t, f)] = |E[T_x(t, f)]|^2 + O\left(\frac{1}{N}\right).$$

The expectation can be expressed by using Equation (11) of the manuscript,

$$E[T_x(t, f)] = E \left[ |T_x(t, f)| e^{i\theta_x(t, f)} \right],$$

and further developed using Equation (6) of the manuscript,

$$E \left[ |T_x(t, f)| e^{i\theta_x(t, f)} \right] = E \left[ e^{i\theta_x(t, f)} \right] E[|T_x(t, f)|] + \text{Cov} \left[ e^{i\theta_x(t, f)}, |T_x(t, f)| \right].$$

Consequently,

$$|E[T_x(t, f)]|^2 = \left| E \left[ e^{i\theta_x(t, f)} \right] E[|T_x(t, f)|] + \text{Cov} \left[ e^{i\theta_x(t, f)}, |T_x(t, f)| \right] \right|^2. \quad (\text{S-55})$$

As a conclusion, we have from (S-54) and (S-55) that

$$\begin{aligned} & E[\text{POWavg}_{x_{1:N}}(t, f)] - E[\text{ITC}_{x_{1:N}}(t, f)^2 \times \text{avgAMP}_{x_{1:N}}(t, f)^2] \\ &= \left| E \left[ e^{i\theta_x(t, f)} \right] E[|T_x(t, f)|] + \text{Cov} \left[ e^{i\theta_x(t, f)}, |T_x(t, f)| \right] \right|^2 - \left| E \left[ e^{i\theta_x(t, f)} \right] \right|^2 E[|T_x(t, f)|]^2 + O\left(\frac{1}{N}\right). \end{aligned} \quad (\text{S-56})$$

This is in general not  $O(1/N)$ . A particular case occurs when

$$\text{Cov} \left[ e^{i\theta_x(t, f)}, |T_x(t, f)| \right] = 0, \quad (\text{S-57})$$

which does make the difference of (S-56)  $O(1/N)$ . Since independence implies a zero covariance, independence of  $e^{i\theta_x(t,f)}$  and  $|T_x(t, f)|$  has the same effect on (S-56). Considering more general solutions is more challenging. For instance, considering the first moments of  $e^{i\theta_x(t,f)}$  and  $|T_x(t, f)|$  fixed, the difference is  $O(1/N)$  only if we have a relation of the form

$$|z - z_0|^2 = r^2,$$

with

$$\begin{aligned} z &= \text{Cov} \left[ e^{i\theta_x(t,f)}, |T_x(t, f)| \right] \\ z_0 &= -\text{E} \left[ e^{i\theta_x(t,f)} \right] \text{E}[|T_x(t, f)|] \\ r &= \left| \text{E} \left[ e^{i\theta_x(t,f)} \right] \right| \text{E}[|T_x(t, f)|]. \end{aligned}$$

The complex numbers  $z$  that respect (3) are on a circle of center  $z_0$  and radius  $r$ . The case of zero covariance mentioned above corresponds to the case  $z = 0$ .

## References

Polyanin, A.D., Manzhirov, A.V., 2007. Handbook of Mathematics for Engineers and Scientists. Chapman & Hall/CRC, Boca Raton.
