# Supplementary material for: Time-frequency analysis of event-related brain recordings: Connecting power of evoked potential and inter-trial coherence
Source: arXiv:2211.08811 ancillary file (2022-11-16)
Supplement: Supplementary file 2 [file Supplement3.pdf]

# Supplementary material #3 for manuscript “Time-frequency analysis of event-related brain recordings: Connecting power of evoked potential and inter-trial coherence”

Jonas Benhamou, Michel Le Van Quyen, and Guillaume Marrelec

## Contents

|          |                                      |          |
|----------|--------------------------------------|----------|
| <b>1</b> | <b>Oscillatory model</b>             | <b>2</b> |
| 1.1      | First result . . . . .               | 2        |
| 1.2      | Second result . . . . .              | 3        |
| <b>2</b> | <b>Proof of general relationship</b> | <b>4</b> |

# 1 Oscillatory model

## 1.1 First result

We here provide bounds for the function

$$t \mapsto \frac{e^{-8\pi^2 \frac{\nu}{f}} \sin(2\phi + 4\pi\nu t)}{1 + e^{-8\pi^2 \frac{\nu}{f}} \cos(2\phi + 4\pi\nu t)}. \quad (\text{S-1})$$

We first set  $b_f = e^{-8\pi^2 \frac{\nu}{f}}$ ,  $u = 2\phi + 4\pi\nu t$  and

$$g(u) = \frac{b_f \sin u}{1 + b_f \cos u}. \quad (\text{S-2})$$

The derivative of  $g$  is given by

$$\begin{aligned} g'(u) &= \frac{b_f \cos u (1 + b_f \cos u) + b_f^2 \sin^2 u}{(1 + b_f \cos u)^2} \\ &= \frac{b_f^2 + b_f \cos u}{(1 + b_f \cos u)^2}. \end{aligned}$$

We therefore have  $g'(u) = 0$  if and only if  $\cos u = -b_f$ , i.e.,  $u = \pm \arccos(-b_f)$ . For  $b_f < 1$ ,  $g'$  is strictly negative on  $[-\pi, -\arccos(-b_f)[$  and  $] \arccos(-b_f), \pi]$ , and strictly positive on  $] -\arccos(-b_f), \arccos(-b_f)[$ . As a consequence,  $g$  is strictly decreasing on  $[-\pi, -\arccos(-b_f)[$  and  $] \arccos(-b_f), \pi]$ , and strictly increasing on  $] -\arccos(-b_f), \arccos(-b_f)[$ . We also have  $g(-\pi) = g(\pi) = 0$ , as well as

$$\begin{aligned} g[\arccos(-b_f)] &= \frac{b_f \sin [\arccos(-b_f)]}{1 + b_f \cos [\arccos(-b_f)]} \\ &= \frac{b_f \sqrt{1 - b_f^2}}{1 - b_f^2} \\ &= \frac{b_f}{\sqrt{1 - b_f^2}} \\ g[-\arccos(-b_f)] &= \frac{b_f \sin [-\arccos(-b_f)]}{1 + b_f \cos [-\arccos(-b_f)]} \\ &= -\frac{b_f}{\sqrt{1 - b_f^2}}. \end{aligned}$$

Setting  $g_f = b_f / \sqrt{1 - b_f^2}$ , we obtain that  $-g_f$  is a lower bound of  $g$ , and  $g_f$  an upper bound. Finally,  $|g(u)| \leq g_f$  for all  $u$ .

## 1.2 Second result

We prove that

$$f \mapsto \arctan \frac{e^{-8\pi^2 \frac{\nu}{f}} \sqrt{1 - e^{-16\pi^2 \frac{\nu}{f}}}}{1 - e^{-16\pi^2 \frac{\nu}{f}}} \quad (\text{S-3})$$

is a strictly increasing function of  $f$ . To show this result, we show that the function is the composition of three functions that are strictly positive. First, it is direct to see that  $f \mapsto e^{-8\pi^2 \frac{\nu}{f}}$  is a strictly increasing function. We then consider

$$h(u) = \frac{u\sqrt{1-u^2}}{1-u^2}. \quad (\text{S-4})$$

Its derivative is given by

$$\begin{aligned} h'(u) &= \frac{\sqrt{1-u^2}}{1-u^2} + \frac{u}{1-u^2} \frac{-2u}{2\sqrt{1-u^2}} + u\sqrt{1-u^2} \frac{2u}{(1-u^2)^2} \\ &= \frac{1}{\sqrt{1-u^2}} + \frac{u^2}{(1-u^2)^{\frac{3}{2}}} \\ &= \frac{1}{(1-u^2)^{\frac{3}{2}}}, \end{aligned}$$

which is positive. So  $h$  is also strictly increasing. Finally,  $u \mapsto \arctan u$  is strictly increasing.

## 2 Proof of general relationship

We expand  $\text{avgAMP}^2 \times \text{ITC}^2$  from Equations (80) and (82) of the manuscript:

$$\begin{aligned}
& \text{avgAMP}_{x_{1:N}}(t, f)^2 \times \text{ITC}_{x_{1:N}}(t, f)^2 \\
&= \frac{1}{N^2} \left[ \sum_{k=1}^N |T_{x_k}(t, f)|^2 + \sum_{k \neq l} |T_{x_k}(t, f)| |T_{x_l}(t, f)| \right] \left\{ \frac{1}{N} + \frac{1}{N^2} \sum_{m \neq n} e^{i[\theta_{x_m}(t, f) - \theta_{x_n}(t, f)]} \right\} \\
&= \underbrace{\frac{1}{N^3} \sum_{k=1}^N |T_{x_k}(t, f)|^2}_{S_1} + \underbrace{\frac{1}{N^3} \sum_{k \neq l} |T_{x_k}(t, f)| |T_{x_l}(t, f)|}_{S_2} + \underbrace{\frac{1}{N^4} \left[ \sum_{k=1}^N |T_{x_k}(t, f)|^2 \right] \left\{ \sum_{m \neq n} e^{i[\theta_{x_m}(t, f) - \theta_{x_n}(t, f)]} \right\}}_{P_1} \\
&\quad + \underbrace{\frac{1}{N^4} \left[ \sum_{k \neq l} |T_{x_k}(t, f)| |T_{x_l}(t, f)| \right] \left\{ \sum_{m \neq n} e^{i[\theta_{x_m}(t, f) - \theta_{x_n}(t, f)]} \right\}}_{P_2}. \tag{S-5}
\end{aligned}$$

$P_1$  of Equation (S-5) needs to be further expanded, yielding

$$\begin{aligned}
P_1 &= \frac{1}{N^4} \sum_{m \neq n} e^{i[\theta_{x_m}(t, f) - \theta_{x_n}(t, f)]} \sum_{k=1}^N |T_{x_k}(t, f)|^2 \\
&= \frac{1}{N^4} \sum_{m \neq n} e^{i[\theta_{x_m}(t, f) - \theta_{x_n}(t, f)]} \left[ |T_{x_m}(t, f)|^2 + |T_{x_n}(t, f)|^2 + \sum_{k \notin \{m, n\}} |T_{x_k}(t, f)|^2 \right] \\
&= \underbrace{\frac{1}{N^4} \sum_{m \neq n} |T_{x_m}(t, f)|^2 e^{i[\theta_{x_m}(t, f) - \theta_{x_n}(t, f)]}}_{S_3} + \underbrace{\frac{1}{N^4} \sum_{m \neq n} |T_{x_n}(t, f)|^2 e^{i[\theta_{x_m}(t, f) - \theta_{x_n}(t, f)]}}_{S_4} + \underbrace{\frac{1}{N^4} \sum_{m \neq n} e^{i[\theta_{x_m}(t, f) - \theta_{x_n}(t, f)]} \sum_{k \notin \{m, n\}} |T_{x_k}(t, f)|^2}_{S_5}. \tag{S-6}
\end{aligned}$$

$P_2$  of Equation (S-5) also needs to be expanded:

$$\begin{aligned}
P_2 &= \frac{1}{N^4} \sum_{m \neq n} e^{i[\theta_{x_m}(t,f) - \theta_{x_n}(t,f)]} \sum_{k \neq l} |T_{x_k}(t,f)| |T_{x_l}(t,f)| \\
&= \frac{1}{N^4} \sum_{m \neq n} e^{i[\theta_{x_m}(t,f) - \theta_{x_n}(t,f)]} \sum_{k=1}^N |T_{x_k}(t,f)| \sum_{l \neq k} |T_{x_l}(t,f)| \\
&= \frac{1}{N^4} \sum_{m \neq n} e^{i[\theta_{x_m}(t,f) - \theta_{x_n}(t,f)]} \left[ |T_{x_m}(t,f)| \sum_{l \neq m} |T_{x_l}(t,f)| + |T_{x_n}(t,f)| \sum_{l \neq n} |T_{x_l}(t,f)| + \sum_{k \notin \{m,n\}} |T_{x_k}(t,f)| \sum_{l \neq k} |T_{x_l}(t,f)| \right] \\
&= \frac{1}{N^4} \sum_{m \neq n} e^{i[\theta_{x_m}(t,f) - \theta_{x_n}(t,f)]} \left\{ |T_{x_m}(t,f)| |T_{x_n}(t,f)| + |T_{x_m}(t,f)| \sum_{l \notin \{m,n\}} |T_{x_l}(t,f)| + |T_{x_n}(t,f)| |T_{x_m}(t,f)| + |T_{x_n}(t,f)| \sum_{l \notin \{m,n\}} |T_{x_l}(t,f)| \right. \\
&\quad \left. + \sum_{l \notin \{m,n\}} |T_{x_l}(t,f)| \left[ |T_{x_m}(t,f)| + |T_{x_n}(t,f)| + \sum_{k \notin \{l,m,n\}} |T_{x_k}(t,f)| \right] \right\} \\
&= \frac{1}{N^4} \sum_{m \neq n} e^{i[\theta_{x_m}(t,f) - \theta_{x_n}(t,f)]} \left[ 2 |T_{x_m}(t,f)| |T_{x_n}(t,f)| + 2 (|T_{x_m}(t,f)| + |T_{x_n}(t,f)|) \sum_{l \notin \{m,n\}} |T_{x_l}(t,f)| + \sum_{l \notin \{m,n\}} |T_{x_l}(t,f)| \sum_{k \notin \{l,m,n\}} |T_{x_k}(t,f)| \right] \\
&= \underbrace{\frac{2}{N^4} \sum_{m \neq n} |T_{x_m}(t,f)| |T_{x_n}(t,f)| e^{i[\theta_{x_m}(t,f) - \theta_{x_n}(t,f)]}}_{S_6} + \underbrace{\frac{2}{N^4} \sum_{m \neq n} |T_{x_m}(t,f)| e^{i[\theta_{x_m}(t,f) - \theta_{x_n}(t,f)]} \sum_{l \notin \{m,n\}} |T_{x_l}(t,f)|}_{S_7} \\
&\quad + \underbrace{\frac{2}{N^4} \sum_{m \neq n} |T_{x_n}(t,f)| e^{i[\theta_{x_m}(t,f) - \theta_{x_n}(t,f)]} \sum_{l \notin \{m,n\}} |T_{x_l}(t,f)|}_{S_8} + \underbrace{\frac{1}{N^4} \sum_{m \neq n} e^{i[\theta_{x_m}(t,f) - \theta_{x_n}(t,f)]} \sum_{l \notin \{m,n\}} |T_{x_l}(t,f)| \sum_{k \notin \{l,m,n\}} |T_{x_k}(t,f)|}_{S_9}. \tag{S-7}
\end{aligned}$$

As a summary, we were able to expand  $\text{avgAMP}_{x_{1:N}}(t,f)^2 \times \text{ITC}_{x_{1:N}}(t,f)^2$  into 9 terms: two ( $S_1$  and  $S_2$ ) from Equation (S-5), three ( $S_3$  to  $S_5$ ) from Equation (S-6), and 4 ( $S_6$  to  $S_9$ ) from Equation (S-7). We can now calculate the expectation of  $\text{avgAMP}_{x_{1:N}}(t,f)^2 \times \text{ITC}_{x_{1:N}}(t,f)^2$  term by term:

- The first term,  $E(S_1)$ , yields

$$\begin{aligned}
E(S_1) &= E \left[ \frac{1}{N^3} \sum_{k=1}^N |T_{x_k}(t, f)|^2 \right] \\
&= \frac{1}{N^3} \sum_{k=1}^N E \left[ |T_{x_k}(t, f)|^2 \right] \\
&= \frac{1}{N^3} \sum_{k=1}^N E \left[ |T_x(t, f)|^2 \right] \\
&= \frac{1}{N^2} E \left[ |T_x(t, f)|^2 \right],
\end{aligned}$$

for a resulting contribution to the general sum that is  $O(1/N^2)$ .

- The second term,  $E(S_2)$ , is equal to

$$\begin{aligned}
E(S_2) &= E \left[ \frac{1}{N^3} \sum_{k \neq l} |T_{x_k}(t, f)| |T_{x_l}(t, f)| \right] \\
&= \frac{1}{N^3} \sum_{k \neq l} E [|T_{x_k}(t, f)| |T_{x_l}(t, f)|] \\
&= \frac{1}{N^3} \sum_{k \neq l} E [|T_{x_k}(t, f)|] E [|T_{x_l}(t, f)|] \\
&= \frac{1}{N^3} \sum_{k \neq l} E [|T_x(t, f)|]^2 \\
&= \frac{N-1}{N^2} E [|T_x(t, f)|]^2,
\end{aligned}$$

for a global contribution that is  $O(1/N)$ .

- The third term,  $E(S_3)$ , is given by

$$\begin{aligned}
E(S_3) &= E \left\{ \frac{1}{N^4} \sum_{m \neq n} |T_{x_m}(t, f)|^2 e^{i[\theta_{x_m}(t, f) - \theta_{x_n}(t, f)]} \right\} \\
&= \frac{1}{N^4} \sum_{m \neq n} E \left\{ |T_{x_m}(t, f)|^2 e^{i[\theta_{x_m}(t, f) - \theta_{x_n}(t, f)]} \right\} \\
&= \frac{1}{N^4} \sum_{m \neq n} E \left[ |T_{x_m}(t, f)|^2 e^{i\theta_{x_m}(t, f)} \right] E \left[ e^{-i\theta_{x_n}(t, f)} \right] \\
&= \frac{1}{N^4} \sum_{m \neq n} E \left[ |T_x(t, f)|^2 e^{i\theta_x(t, f)} \right] E \left[ e^{-i\theta_x(t, f)} \right] \\
&= \frac{N-1}{N^3} E \left[ |T_x(t, f)|^2 e^{i\theta_x(t, f)} \right] E \left[ e^{i\theta_x(t, f)} \right]^*,
\end{aligned}$$

which is  $O(1/N^2)$ .

- The fourth term,  $E(S_4)$ , is similar to the previous,

$$\begin{aligned}
E(S_4) &= E \left\{ \frac{1}{N^4} \sum_{m \neq n} |T_{x_n}(t, f)|^2 e^{i[\theta_{x_m}(t, f) - \theta_{x_n}(t, f)]} \right\} \\
&= \frac{N-1}{N^3} E \left[ |T_x(t, f)|^2 e^{i\theta_x(t, f)} \right]^* E \left[ e^{i\theta_x(t, f)} \right],
\end{aligned}$$

which is also  $O(1/N^2)$ .

- The fifth term,  $E(S_5)$ , yields

$$\begin{aligned}
E(S_5) &= E \left\{ \frac{1}{N^4} \sum_{m \neq n} e^{i[\theta_{x_m}(t,f) - \theta_{x_n}(t,f)]} \sum_{k \notin \{m,n\}} |T_{x_k}(t,f)|^2 \right\} \\
&= \frac{1}{N^4} \sum_{m \neq n} E \left\{ e^{i[\theta_{x_m}(t,f) - \theta_{x_n}(t,f)]} \sum_{k \notin \{m,n\}} |T_{x_k}(t,f)|^2 \right\} \\
&= \frac{1}{N^4} \sum_{m \neq n} E \left[ e^{i\theta_{x_m}(t,f)} \right] E \left[ e^{-i\theta_{x_n}(t,f)} \right] E \left[ \sum_{k \notin \{m,n\}} |T_{x_k}(t,f)|^2 \right] \\
&= \frac{1}{N^4} \sum_{m \neq n} E \left[ e^{i\theta_{x_m}(t,f)} \right] E \left[ e^{i\theta_{x_n}(t,f)} \right]^* \sum_{k \notin \{m,n\}} E \left[ |T_{x_k}(t,f)|^2 \right] \\
&= \frac{1}{N^4} \sum_{m \neq n} E \left[ e^{i\theta_x(t,f)} \right] E \left[ e^{i\theta_x(t,f)} \right]^* \sum_{k \notin \{m,n\}} E \left[ |T_x(t,f)|^2 \right] \\
&= \frac{N(N-1)(N-2)}{N^4} E \left[ |T_x(t,f)|^2 \right] \left| E \left[ e^{i\theta_x(t,f)} \right] \right|^2 \\
&= \frac{(N-1)(N-2)}{N^3} E \left[ |T_x(t,f)|^2 \right] \left| E \left[ e^{i\theta_x(t,f)} \right] \right|^2,
\end{aligned}$$

which is  $O(1/N)$ .

- The sixth term,  $E(S_6)$ , yields

$$\begin{aligned}
S_6 &= E \left\{ \frac{2}{N^4} \sum_{m \neq n} |T_{x_m}(t, f)| |T_{x_n}(t, f)| e^{i[\theta_{x_m}(t, f) - \theta_{x_n}(t, f)]} \right\} \\
&= \frac{2}{N^4} \sum_{m \neq n} E \left\{ |T_{x_m}(t, f)| |T_{x_n}(t, f)| e^{i[\theta_{x_m}(t, f) - \theta_{x_n}(t, f)]} \right\} \\
&= \frac{2}{N^4} \sum_{m \neq n} E \left[ |T_{x_m}(t, f)| e^{i\theta_{x_m}(t, f)} \right] E \left[ |T_{x_n}(t, f)| e^{-i\theta_{x_n}(t, f)} \right] \\
&= \frac{2}{N^4} \sum_{m \neq n} E [T_{x_m}(t, f)] E [T_{x_n}(t, f)^*] \\
&= \frac{2}{N^4} \sum_{m \neq n} E [T_x(t, f)] E [T_x(t, f)]^* \\
&= \frac{2}{N^4} \sum_{m \neq n} |E [T_x(t, f)]|^2 \\
&= \frac{2N(N-1)}{N^4} |E [T_x(t, f)]|^2 \\
&= \frac{2(N-1)}{N^3} |E [T_x(t, f)]|^2,
\end{aligned}$$

which is  $O(1/N^2)$ .

- The seventh term,  $E(S_7)$ , yields

$$\begin{aligned}
E(S_7) &= E \left\{ \frac{2}{N^4} \sum_{m \neq n} |T_{x_m}(t, f)| e^{i[\theta_{x_m}(t, f) - \theta_{x_n}(t, f)]} \sum_{l \notin \{m, n\}} |T_{x_l}(t, f)| \right\} \\
&= \frac{2}{N^4} \sum_{m \neq n} E \left\{ |T_{x_m}(t, f)| e^{i[\theta_{x_m}(t, f) - \theta_{x_n}(t, f)]} \sum_{l \notin \{m, n\}} |T_{x_l}(t, f)| \right\} \\
&= \frac{2}{N^4} \sum_{m \neq n} E \left[ |T_{x_m}(t, f)| e^{i\theta_{x_m}(t, f)} \right] E \left[ e^{-i\theta_{x_n}(t, f)} \right] E \left[ \sum_{l \notin \{m, n\}} |T_{x_l}(t, f)| \right] \\
&= \frac{2}{N^4} \sum_{m \neq n} E [T_{x_m}(t, f)] E \left[ e^{i\theta_{x_n}(t, f)} \right]^* \sum_{l \notin \{m, n\}} E [|T_{x_l}(t, f)|] \\
&= \frac{2}{N^4} \sum_{m \neq n} E [T_x(t, f)] E \left[ e^{i\theta_x(t, f)} \right]^* \sum_{l \notin \{m, n\}} E [|T_x(t, f)|] \\
&= \frac{2N(N-1)(N-2)}{N^4} E [T_x(t, f)] E \left[ e^{i\theta_x(t, f)} \right]^* E [|T_x(t, f)|] \\
&= \frac{2(N-1)(N-2)}{N^3} E [T_x(t, f)] E \left[ e^{i\theta_x(t, f)} \right]^* E [|T_x(t, f)|],
\end{aligned}$$

which is  $O(1/N)$ .

- The eight term,  $E(S_8)$ , yields

$$\begin{aligned}
E(S_8) &= E \left\{ \frac{2}{N^4} \sum_{m \neq n} |T_{x_n}(t, f)| e^{i[\theta_{x_m}(t, f) - \theta_{x_n}(t, f)]} \sum_{l \notin \{m, n\}} |T_{x_l}(t, f)| \right\} \\
&= \frac{2}{N^4} \sum_{m \neq n} E \left\{ |T_{x_n}(t, f)| e^{i[\theta_{x_m}(t, f) - \theta_{x_n}(t, f)]} \sum_{l \notin \{m, n\}} |T_{x_l}(t, f)| \right\} \\
&= \frac{2}{N^4} \sum_{m \neq n} E \left[ |T_{x_n}(t, f)| e^{-i\theta_{x_n}(t, f)} \right] E \left[ e^{i\theta_{x_m}(t, f)} \right] E \left[ \sum_{l \notin \{m, n\}} |T_{x_l}(t, f)| \right] \\
&= \frac{2}{N^4} \sum_{m \neq n} E [T_{x_n}(t, f)^*] E \left[ e^{i\theta_{x_m}(t, f)} \right] \sum_{l \notin \{m, n\}} E [|T_{x_l}(t, f)|] \\
&= \frac{2}{N^4} \sum_{m \neq n} E [T_x(t, f)^*] E \left[ e^{i\theta_x(t, f)} \right] \sum_{l \notin \{m, n\}} E [|T_x(t, f)|] \\
&= \frac{2N(N-1)(N-2)}{N^4} E [T_x(t, f)^*] E \left[ e^{i\theta_x(t, f)} \right] E [|T_x(t, f)|] \\
&= \frac{2(N-1)(N-2)}{N^3} E [T_x(t, f)^*] E \left[ e^{i\theta_x(t, f)} \right] E [|T_x(t, f)|],
\end{aligned}$$

which is  $O(1/N)$ .

- Finally, the ninth term,  $E(S_9)$ , yields

$$\begin{aligned}
E(S_9) &= E \left\{ \frac{1}{N^4} \sum_{m \neq n} e^{i[\theta_{x_m}(t,f) - \theta_{x_n}(t,f)]} \sum_{l \notin \{m,n\}} |T_{x_l}(t,f)| \sum_{k \notin \{l,m,n\}} |T_{x_k}(t,f)| \right\} \\
&= \frac{1}{N^4} \sum_{m \neq n} E \left\{ e^{i[\theta_{x_m}(t,f) - \theta_{x_n}(t,f)]} \sum_{l \notin \{m,n\}} |T_{x_l}(t,f)| \sum_{k \notin \{l,m,n\}} |T_{x_k}(t,f)| \right\} \\
&= \frac{1}{N^4} \sum_{m \neq n} E \left[ e^{i\theta_{x_m}(t,f)} \right] E \left[ e^{-i\theta_{x_n}(t,f)} \right] E \left[ \sum_{l \notin \{m,n\}} |T_{x_l}(t,f)| \sum_{k \notin \{l,m,n\}} |T_{x_k}(t,f)| \right] \\
&= \frac{1}{N^4} \sum_{m \neq n} E \left[ e^{i\theta_{x_m}(t,f)} \right] E \left[ e^{i\theta_{x_n}(t,f)} \right]^* \sum_{l \notin \{m,n\}} E \left[ |T_{x_l}(t,f)| \sum_{k \notin \{l,m,n\}} |T_{x_k}(t,f)| \right] \\
&= \frac{1}{N^4} \sum_{m \neq n} E \left[ e^{i\theta_{x_m}(t,f)} \right] E \left[ e^{i\theta_{x_n}(t,f)} \right]^* \sum_{l \notin \{m,n\}} E [|T_{x_l}(t,f)|] E \left[ \sum_{k \notin \{l,m,n\}} |T_{x_k}(t,f)| \right] \\
&= \frac{1}{N^4} \sum_{m \neq n} E \left[ e^{i\theta_{x_m}(t,f)} \right] E \left[ e^{i\theta_{x_n}(t,f)} \right]^* \sum_{l \notin \{m,n\}} E [|T_{x_l}(t,f)|] \sum_{k \notin \{l,m,n\}} E [|T_{x_k}(t,f)|] \\
&= \frac{1}{N^4} \sum_{m \neq n} E \left[ e^{i\theta_x(t,f)} \right] E \left[ e^{i\theta_x(t,f)} \right]^* \sum_{l \notin \{m,n\}} E [|T_x(t,f)|] \sum_{k \notin \{l,m,n\}} E [|T_x(t,f)|] \\
&= \frac{1}{N^4} \sum_{m \neq n} \left| E \left[ e^{i\theta_x(t,f)} \right] \right|^2 \sum_{l \notin \{m,n\}} E [|T_x(t,f)|] \sum_{k \notin \{l,m,n\}} E [|T_x(t,f)|] \\
&= \frac{N(N-1)(N-2)(N-3)}{N^4} \left| E \left[ e^{i\theta_x(t,f)} \right] \right|^2 E [|T_x(t,f)|]^2 \\
&= \frac{(N-1)(N-2)(N-3)}{N^3} \left| E \left[ e^{i\theta_x(t,f)} \right] \right|^2 E [|T_x(t,f)|]^2.
\end{aligned}$$

This is the only term that is  $O(1)$ .

Putting all calculations together, we obtain the following

$$\begin{aligned}
\mathbb{E}(\text{avgAMP}^2 \times \text{ITC}^2) &= \mathbb{E} \left[ \sum_{i=1}^9 S_i \right] \\
&= \sum_{i=1}^9 \mathbb{E}[S_i] \\
&= \frac{(N-1)(N-2)(N-3)}{N^3} \left| \mathbb{E} \left[ e^{i\theta_x(t,f)} \right] \right|^2 \mathbb{E} [|T_x(t, f)|]^2 + O \left( \frac{1}{N} \right) \\
&= \left( 1 - \frac{1}{N} \right) \left( 1 - \frac{2}{N} \right) \left( 1 - \frac{3}{N} \right) \left| \mathbb{E} \left[ e^{i\theta_x(t,f)} \right] \right|^2 \mathbb{E} [|T_x(t, f)|]^2 + O \left( \frac{1}{N} \right) \\
&= \left| \mathbb{E} \left[ e^{i\theta_x(t,f)} \right] \right|^2 \mathbb{E} [|T_x(t, f)|]^2 + O \left( \frac{1}{N} \right).
\end{aligned}$$
